# Supplementary material for: Quantum Nonlinear Optics in Atomically Thin Materials
Source: arXiv:1805.04805 ancillary file (2018-09-23)
Supplement: Supplementary file 1 [file supplementary.pdf]

# Supplemental Material: Quantum Nonlinear Optics in an Atomically Thin Material Proximal to a Mirror

Dominik S. Wild,[1] Ephraim Shahmoon,[1] Susanne F. Yelin,[1,2] and Mikhail D. Lukin[1]

[1]Department of Physics, Harvard University, Cambridge, MA 02138, USA

[2]Department of Physics, University of Connecticut, Storrs, CT 06269, USA

## I. LINEAR RESPONSE

The reflection and transmission coefficients of a TMD (or any other two-dimensional, resonant emitter) are given by [S1]

$$r_{\mathrm{TMD}}(\delta) = -\frac{i\gamma/2}{\delta + i(\gamma+\gamma')/2}, \qquad t_{\mathrm{TMD}}(\delta) = \frac{\delta + i\gamma'/2}{\delta + i(\gamma+\gamma')/2}. \tag{S1}$$

The transmission and reflection coefficients for the entire system, including the mirror, can be obtained by summing over all multiple reflection processes:

$$r(\delta) = r_{\mathrm{TMD}}(\delta) + t_{\mathrm{TMD}}(\delta)^2 r_0 e^{2ikd}\left[1 + r_{\mathrm{TMD}}(\delta) r_0 e^{2ikd} + r_{\mathrm{TMD}}(\delta)^2 r_0^2 e^{4ikd} + \cdots\right], \tag{S2}$$

$$t(\delta) = t_{\mathrm{TMD}}(\delta)\left[1 + r_{\mathrm{TMD}}(\delta) r_0 e^{2ikd} + r_{\mathrm{TMD}}(\delta)^2 r_0^2 e^{4ikd} + \cdots\right] t_0 e^{ikd}. \tag{S3}$$

Here, $k = k_0 + \delta/c$ is the wavenumber of the incident light. By evaluating the geometric sums, we obtain

$$r(\delta) = r_0 e^{2ikd} - \frac{i\gamma/2(1 + r_0 e^{2ikd})^2}{\delta + i\gamma/2(1 + r_0 e^{2ikd}) + i\gamma'/2}, \tag{S4}$$

$$t(\delta) = \frac{\delta + i\gamma'/2}{\delta + i\gamma/2(1 + r_0 e^{2ikd}) + i\gamma'/2} t_0 e^{ikd}. \tag{S5}$$

It is easily verified that perfect transmission (zero reflection) occurs when $\gamma' = 0$, $\delta = \pm(\gamma/2)|t_0|/|r_0|$, and $r_0 e^{2ikd} = -|r_0|^2 \pm i|r_0||t_0|$.

## II. HEISENBERG–LANGEVIN EQUATION

We derive a Heisenberg–Langevin equation for a two-dimensional emitter in front of a partially reflecting mirror (Eq. (1) of the main text). If the system is translationally invariant in the plane of the emitter, conservation of momentum allows us to consider each in-plane momentum component separately. The Hamiltonian for the zero-momentum components is given by

$$H = H_0 + \sum_k \omega_k d_k^\dagger d_k + i\sum_k g_k\left(d_k^\dagger a - a^\dagger d_k\right), \tag{S6}$$

where $a$ is the annihilation operator of a delocalized excitations (excitons in case of a TMD) and $d_k$ is the photon annihilation operators for a plane-wave mode with momentum $k$ normal to the mirror and the emitter. At this stage, the Hamiltonian only includes free-space photonic modes. The mirror will be introduced below by imposing suitable boundary conditions. We expect the form of the Hamiltonian to remain valid to a good approximation for a finite-sized system if the incident beam is chosen such that only a single transverse mode needs to be taken into account at the location of the emitter. In this case, the operators $a$ and $d_k$ correspond to states whose transverse profile is determined by the incident light. A correction to this picture due to exciton dispersion is discussed in the main text.

Following the input–output formalism in reference [S2], we make the Markov approximation, $g_k \approx \sqrt{\gamma/2}$, within which the evolution of some system operator $Q$ may be written as

$$\begin{aligned}\dot{Q} = &-i\left[Q, H_0\right] + \gamma\left(a^\dagger Q a - \frac{1}{2}\left\{Q, a^\dagger a\right\}\right) \\ &+ \sqrt{\frac{\gamma}{2}}\left(b_{\mathrm{in},R}^\dagger\left[Q, a\right] - \left[Q, a^\dagger\right] b_{\mathrm{in},R}\right) + \sqrt{\frac{\gamma}{2}}\left(c_{\mathrm{in}}^\dagger\left[Q, a\right] - \left[Q, a^\dagger\right] c_{\mathrm{in}}\right),\end{aligned} \tag{S7}$$

where the input fields are defined as

$$b_{\mathrm{in},R}(t) = \sum_{k>0} d_k(t_0) e^{-i\omega_k (t-t_0)}, \qquad c_{\mathrm{in}}(t) = \sum_{k<0} d_k(t_0) e^{-i\omega_k (t-t_0)} \tag{S8}$$

for an early time $t_0 \to -\infty$. In order to account for the mirror, we apply boundary conditions to the electric field. The electric field is computed within the Markov approximation assuming a linear dispersion relation $\omega_k = kc$. For the field propagating to the right, we obtain

$$E_R^+(z,t) \propto \sum_{k>0} g_k d_k(t) e^{ikz} \propto \begin{cases} b_{\mathrm{in},R}(t-z/c) & \text{if } z<0 \\ c_{\mathrm{out}}(t-z/c) & \text{if } 0<z<d \\ b_{\mathrm{out},R}(t-(z-d)/c) & \text{if } d<z \end{cases}, \tag{S9}$$

while for left-moving modes

$$E_L^+(z,t) \propto \sum_{k<0} g_k d_k(t) e^{ikz} \propto \begin{cases} b_{\mathrm{out},L}(t+z/c) & \text{if } z<0 \\ c_{\mathrm{in}}(t+z/c) & \text{if } 0<z<d \\ b_{\mathrm{in},L}(t+(z-d)/c) & \text{if } d<z \end{cases}. \tag{S10}$$

Here we introduced

$$c_{\mathrm{out}}(t) = b_{\mathrm{in},R}(t) + \sqrt{\frac{\gamma}{2}} a(t), \qquad b_{\mathrm{out},L}(t) = c_{\mathrm{in}}(t) + \sqrt{\frac{\gamma}{2}} a(t). \tag{S11}$$

The operators $b_{\mathrm{out},R}$ and $b_{\mathrm{in},L}$ correspond to the field to the right of the mirror. They are determined by the boundary conditions at the mirror,

$$c_{\mathrm{in}}(t) = r_0 c_{\mathrm{out}}(t-2d/c) + t_0 b_{\mathrm{in},L}(t-d/c), \qquad b_{\mathrm{out},R}(t) = t_0 c_{\mathrm{out}}(t-d/c) - \frac{t_0}{t_0^*} r_0^* b_{\mathrm{in},L}(t), \tag{S12}$$

where we used the fact that for a nonabsorbing mirror, the transmission coefficients from both sides are identical, while the reflection coefficient from the right is $-t_0 r_0^*/t_0^*$, given the reflection coefficient $r_0$ from the left. Figure S1 illustrates the physical interpretation of the various photon operators.

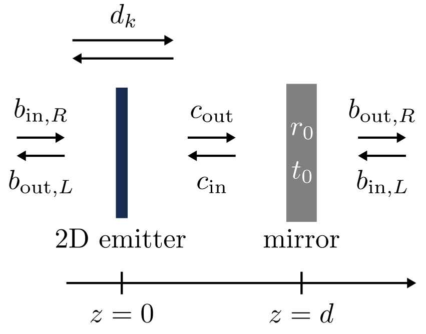


FIG. S1. Photon operators used in the input–output formalism.

The dynamics of the system and the electric field are in principle fully determined by Eqs. S7, S11, and S12 along with initial conditions for the input fields $b_{\mathrm{in},R}$ and $b_{\mathrm{in},L}$. However, the equations are nonlocal in time, which renders them difficult to solve. To turn them into local equations, we neglect retardation, $a(t-2d/c) \approx e^{2ik_0 d} a(t)$, and we assume that the input field is sufficiently narrow band such that $b_{\mathrm{in},R}(t-2d/c) \approx e^{2ik_0 d} b_{\mathrm{in},R}(t)$ and $b_{\mathrm{in},L}(t-2d/c) \approx e^{2ik_0 d} b_{\mathrm{in},L}(t)$. The validity of these approximations will be discussed below. Substituting back into Eq. (S7) yields the Heisenberg–Langevin equation

$$\begin{aligned} \dot{Q} = &-i\left[Q, H_0 + \frac{\gamma}{2} \mathrm{Im}\left(r_0 e^{2ik_0 d}\right) a^\dagger a\right] + \gamma\left[1 + \mathrm{Re}\left(r_0 e^{2ik_0 d}\right)\right]\left(a^\dagger Q a - \frac{1}{2}\left\{Q, a^\dagger a\right\}\right) \\ &- \sqrt{\frac{\gamma}{2}}\left(\left[Q, a^\dagger\right]\left(1 + r_0 e^{2ik_0 d}\right) b_{\mathrm{in},R} + \mathrm{h.c.}\right) - \sqrt{\frac{\gamma}{2}}\left(\left[Q, a^\dagger\right] t_0 e^{ik_0 d} b_{\mathrm{in},L} + \mathrm{h.c.}\right), \end{aligned} \tag{S13}$$

which is supplemented by the input–output relations

$$b_{\mathrm{out},R}(t) = t_0 e^{ik_0 d} b_{\mathrm{in},R}(t) - \frac{t_0}{t_0^*} r_0^* b_{\mathrm{in},L}(t) + \sqrt{\frac{\gamma}{2}} t_0 e^{ik_0 d} a(t), \tag{S14}$$

$$b_{\mathrm{out},L}(t) = r_0 e^{2ik_0 d} b_{\mathrm{in},R}(t) + t_0 e^{ik_0 d} b_{\mathrm{in},L}(t) + \sqrt{\frac{\gamma}{2}} \left(1 + r_0 e^{2ik_0 d}\right) a(t). \tag{S15}$$

For all remaining calculations, we assume that the input fields are prepared in a coherent states. It is then convenient to write the Heisenberg–Langevin equation as

$$\dot{Q} = -i \left[Q, H_0 + \frac{\gamma}{2} \operatorname{Im}\left(r_0 e^{2ik_0 d}\right) a^\dagger a - i \left(\Omega a^\dagger - \Omega^* a\right)\right] + \gamma \left[1 + \operatorname{Re}\left(r_0 e^{2ik_0 d}\right)\right] a^\dagger Q a - \frac{1}{2} \left[Q, a^\dagger a\right] + \mathcal{F}_Q \tag{S16}$$

where we defined the Rabi frequency

$$\Omega = \sqrt{\frac{\gamma}{2}} \left(1 + r_0 e^{2ik_0 d}\right) \langle b_{\mathrm{in},R}\rangle + \sqrt{\frac{\gamma}{2}} t_0 e^{ik_0 d} \langle b_{\mathrm{in},L}\rangle \tag{S17}$$

and the Langevin noise term

$$\mathcal{F}_Q = -\sqrt{\frac{\gamma}{2}} \left(\left[Q, a^\dagger\right] \left(1 + r_0 e^{2ik_0 d}\right) \left(b_{\mathrm{in},R} - \langle b_{\mathrm{in},R}\rangle\right) + \mathrm{h.c.}\right) - \sqrt{\frac{\gamma}{2}} \left(\left[Q, a^\dagger\right] t_0 e^{ik_0 d} (b_{\mathrm{in},L} - \langle b_{\mathrm{in},L}\rangle) + \mathrm{h.c.}\right). \tag{S18}$$

The Langevin noise term has the important property $\langle \mathcal{F}_Q \rangle = 0$ for any $Q$. We have thus arrived at Eq. (1) of the main text up to the additional dissipative terms $\gamma'$ and $\chi_2$.

We next comment of the validity of the Heisenberg–Langevin equation. The Markov approximation $g_k \approx \sqrt{\gamma/2}$ requires that $g_k$ varies little over the range $\omega_0 \pm \gamma$. In free space, this leads to the conditions $\gamma \ll \omega_0$, which is typically satisfied for optical transitions and for TMDs in particular. To understand the conditions under which it is justified to neglect retardation, we switch to a frame that rotates according to

$$a(t) = \tilde{a}(t) e^{-i\omega_0 t}. \tag{S19}$$

We can then expand

$$a(t - 2d/c) \approx \left[\tilde{a}(t) - \frac{2d}{c} \dot{\tilde{a}}(t)\right] e^{-i\omega_0 (t - 2d/c)}. \tag{S20}$$

The magnitude of $\dot{\tilde{a}}$ compared to $\tilde{a}$ is given by $1/\tau_S$, where $\tau_S$ denotes the typical timescale over which the system evolves nontrivially. By following the derivation that led to the Heisenberg–Langevin equation, we obtain a relative correction of order $\gamma d / c\tau_S$. The correction can be certainly neglected if it is smaller than the decay rate, which leads to the condition

$$\frac{1}{\tau_S} \ll \left[1 + \operatorname{Re}\left(r_0 e^{2ik_0 d}\right)\right] \nu_{\mathrm{FSR}}. \tag{S21}$$

There are four frequency scales that determine the time scale of the system: the detuning $\delta$, the Lamb shift $(\gamma/2) \operatorname{Im}\left(r_0 e^{2ik_0 d}\right)$, the decay rate $\gamma \left[1 + \operatorname{Re}\left(r_0 e^{2ik_0 d}\right)\right]$, and the nonlinearity $\chi_{1,2}$. By taking the detuning to be comparable to the Lamb shift, we obtain the three conditions

$$\gamma \ll \frac{1 + \operatorname{Re}\left(r_0 e^{2ik_0 d}\right)}{\left|\operatorname{Im}\left(r_0 e^{2ik_0 d}\right)\right|} \nu_{\mathrm{FSR}}, \qquad \gamma \ll \nu_{\mathrm{FSR}}, \qquad \chi_{1,2} \ll \left[1 + \operatorname{Re}\left(r_0 e^{2ik_0 d}\right)\right] \nu_{\mathrm{FSR}}. \tag{S22}$$

A similar argument can be applied to the input fields, showing that their time dependence can be approximated as $\sim e^{-i\omega_0 t}$ provided the bandwidth and, again, the detuning, are small compared to $\left[1 + \operatorname{Re}\left(r_0 e^{2ik_0 d}\right)\right] \nu_{\mathrm{FSR}}$.

At the Fabry–Pérot resonance, we have $r_0 e^{2ik_0 d} = -R_0 \pm i\sqrt{R_0 T_0}$, which yields two sufficient conditions:

$$\gamma \ll \sqrt{\frac{T_0}{R_0}} \nu_{\mathrm{FSR}}, \qquad \chi_{1,2} \ll T_0 \nu_{\mathrm{FSR}} \tag{S23}$$

With a wavelength scale separation between the TMD and the mirror ($\nu_{\mathrm{FSR}} \sim \omega_0$), both conditions are readily met for the values of $T_0$ required to achieve antibunching.

## III. PHOTON STATISTICS

We may use the input–output relations to relate expectation values and correlation functions of the output field to functions of system operators. For simplicity, let us assume that there is no incident field from the right, while the field incident from the left is in a coherent state. It is convenient to introduce the scaled operators

$$a_L = \frac{(1+r_0 e^{2ik_0 d})^2}{r_0 e^{2ik_0 d}} \frac{a}{2\Omega/\gamma}, \qquad a_R = (1+r_0 e^{2ik_0 d}) \frac{a}{2\Omega/\gamma}, \tag{S24}$$

where the Rabi frequency $\Omega$ is defined in Eq. (S17). The intensity reflection and transmission coefficients may then be expressed as

$$R = \frac{\langle b^\dagger_{\text{out},L} b_{\text{out},L}\rangle}{\langle b^\dagger_{\text{in},R} b_{\text{in},R}\rangle} = \left[1 + \langle a_L\rangle + \langle a_L^\dagger\rangle + \langle a_L^\dagger a_L\rangle\right] R_0, \tag{S25}$$

$$T = \frac{\langle b^\dagger_{\text{out},R} b_{\text{out},R}\rangle}{\langle b^\dagger_{\text{in},R} b_{\text{in},R}\rangle} = \left[1 + \langle a_R\rangle + \langle a_R^\dagger\rangle + \langle a_R^\dagger a_R\rangle\right] T_0. \tag{S26}$$

It is straightforward to show that these expressions agree with the classical result in Eq. (S4) and Eq. (S5) in linear response ($\chi_1 = \chi_2 = 0$) under the same conditions for which the Heisenberg–Langevin equation is valid. For higher-order correlation functions, it is helpful to note that input fields at later times commute with output fields at earlier times, e.g. $[b_{\text{in},R}(t), b_{\text{out},R}(0)] = 0$ for $t > 0$, as a consequence of causality [S2]. In the main text, we are interested in the normalized two-time correlation function of the transmitted light, which thus evaluates to

$$\begin{aligned} g_T^{(2)}(t) &= \frac{\langle b^\dagger_{\text{out},R}(0) b^\dagger_{\text{out},R}(t) b_{\text{out},R}(t) b_{\text{out},R}(0)\rangle}{\langle b^\dagger_{\text{out},R}(0) b_{\text{out},R}(0)\rangle \langle b^\dagger_{\text{out},R}(t) b_{\text{out},R}(t)\rangle} \\ &= \left(\frac{T_0}{T}\right)^2 \Big\{ 1 + 2\left[\langle a_R(0)\rangle + \text{c.c.}\right] + \Big[\langle a_R(t) a_R(0)\rangle + \langle a_R^\dagger(0) a_R(t)\rangle + \langle a_R^\dagger(0) a_R(0)\rangle + \text{c.c.}\Big] \\ &\qquad + \Big[\langle a_R^\dagger(t) a_R(t) a_R(0)\rangle + \langle a_R^\dagger(0) a_R(t) a_R(0)\rangle + \text{c.c.}\Big] + \langle a_R^\dagger(0) a_R^\dagger(t) a_R(t) a_R(0)\rangle \Big\}. \end{aligned} \tag{S27}$$

## IV. ANHARMONIC OSCILLATOR

Above we have shown how to compute the properties of the scattered field when the dynamics of the system are known. We now briefly outline how to obtain the relevant correlation functions for the anharmonic oscillator described in the main text. The Hamiltonian in the rotating frame is given by

$$H = (\Delta - \delta) a^\dagger a + \frac{\chi_1}{2} a^\dagger a^\dagger a a - i\left(\Omega a^\dagger - \Omega^* a\right). \tag{S28}$$

while the nonunitary evolution is captured by the sum of the three dissipators

$$\mathcal{D}_0[Q] = \Gamma\left(a^\dagger Q a - \frac{1}{2}\left\{Q, a^\dagger a\right\}\right) \qquad \text{(linear decay)}, \tag{S29}$$

$$\mathcal{D}_1[Q] = \frac{\chi_2}{2}\left(a^\dagger a^\dagger Q a a - \frac{1}{2}\left\{Q, a^\dagger a^\dagger a a\right\}\right) \qquad \text{(nonlinear decay)}, \tag{S30}$$

$$\mathcal{D}_2[Q] = 2\gamma_d\left(a^\dagger a Q a^\dagger a - \frac{1}{2}\left\{Q, a^\dagger a a^\dagger a\right\}\right) \qquad \text{(pure dephasing)}, \tag{S31}$$

where we defined

$$\Delta = \frac{\gamma}{2}\,\text{Im}\left(r_0 e^{2ik_0 d}\right), \qquad \Gamma = \tilde{\gamma} + \gamma' = \gamma\left[1 + \text{Re}\left(r_0 e^{2ik_0 d}\right)\right] + \gamma'. \tag{S32}$$

In addition to the linear and nonlinear decay terms, which were discussed in detail in the main text, we included the dissipator $\mathcal{D}_2[Q]$ corresponding to pure dephasing at rate $\gamma_d$.

The time evolution of the oscillator is fully determined by the normal ordered expectation values $\langle a^{\dagger\, m} a^n \rangle$. A straightforward calculation yields

$$\begin{aligned}\frac{\mathrm{d}}{\mathrm{d}t}\langle a^{\dagger\, m} a^n \rangle = &- \Big[ i(n-m)(\Delta-\delta) + (n+m)\frac{\Gamma}{2} + i(n(n-1) - m(m-1))\frac{\chi_1}{2} \\ &\qquad + (n(n-1)+m(m-1))\frac{\chi_2}{4} + (n-m)^2\gamma_d \Big] \langle a^{\dagger\, m} a^n \rangle \\ &- n\Omega \langle a^{\dagger\, m} a^{n-1} \rangle - m\Omega^* \langle a^{\dagger\, m-1} a^n \rangle - \Big[ i(n-m)\chi_1 + (n+m)\frac{\chi_2}{2} \Big] \langle a^{\dagger\, m+1} a^{n+1} \rangle. \end{aligned} \tag{S33}$$

We can cast the above equations of motion into matrix form as

$$\frac{\mathrm{d}}{\mathrm{d}t}\langle a^{\dagger\, m} a^n \rangle = \sum_{kl} M_{mn,kl} \langle a^{\dagger\, k} a^l \rangle \tag{S34}$$

To find the steady state, we note that $\langle a^{\dagger\, 0} a^0 \rangle = 1$, which allows us to re-write the equation as

$$M_{mn,00} + \sum_{(k,l)\neq(0,0)} M_{mn,kl} \langle a^{\dagger\, k} a^l \rangle = 0. \tag{S35}$$

Assuming that there exists a unique steady state, as is the case for weak driving, we can numerically solve this equation by matrix inversion in a truncated Fock space.

Once all the normal ordered expectation values are known, two-time correlation functions can be obtained using the quantum regression theorem (valid within the Markov approximation) [S3]. Applied to our problem, the quantum regression theorem states that

$$\frac{\mathrm{d}}{\mathrm{d}t}\langle a^\dagger(0)^p a^\dagger(t)^m a(t)^n a(0)^q \rangle = \sum_{kl} M_{mn,kl} \langle a^\dagger(0)^p a^\dagger(t)^k a(t)^l a(0)^q \rangle, \tag{S36}$$

which can be readily integrated in a truncated Fock space with the initial conditions determined by the steady-state solution. Hence, the two-time correlation functions directly follow from the one-time expectation values.

## V. PURE DEPHASING

In the main text, we discussed the role of loss and provided an upper bound on the loss rate $\gamma'$ for the quantum nonlinearity to be observable. In addition to loss, excitons may also be subject to pure dephasing as described by the dissipative term Eq. (S31). To explore the impact of pure dephasing, we show in Fig. S2 plots analogous to Fig. 1e and Fig. 2d of the main text, replacing the loss rate $\gamma'$ by the dephasing rate $\gamma_d$. The figures clearly indicate that pure dephasing affects the linear and nonlinear response of the system in a qualitatively and quantitatively similar fashion to loss. Hence, the system parameters must satisfy

$$\chi > T_0\gamma > \gamma_d \tag{S37}$$

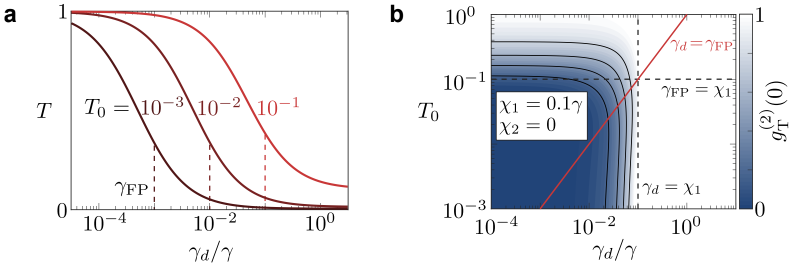


FIG. S2. (a) Transmission at the Fabry–Pérot resonance as a function of the dephasing rate $\gamma_d$, c.f. Fig. 1e of the main text. (b) $g_T^{(2)}(0)$ as a function of $\gamma_d$ and the transmission coefficient $T_0$ of the mirror in analogy with Fig. 2d of the main text. We set $\gamma' = 0$ in both cases.

as well as Eq. (6) of the main text in order to exhibit strong quantum nonlinear dynamics.

[S1] S. Zeytinoğlu, C. Roth, S. Huber, and A. İmamoğlu, Phys. Rev. A **96**, 031801 (2017).
[S2] C. W. Gardiner and M. J. Collett, Phys. Rev. A **31**, 3761 (1985).
[S3] P. Meystre and M. Sargent, *Elements of Quantum Optics* (Springer Berlin Heidelberg, Berlin, Heidelberg, 2007).
